# Supplementary material for: Contextual Emotion Recognition using Large Vision Language Models
Source: arXiv:2405.08992 source file (2025-01-31)
Supplement: Supplementary file 1 [file supplementary.tex]

\subsection{How we should pick the physical signals to describe \textit{how}?} To answer this question we evaluated different thresholding methods on the validation set. After obtaining probabilities from CLIP, we picked the top 1, 3, or 5 physical signals with highest probabilities to generate captions and record the mAP. As the second approach, we picked all the signals which had the probability greater than $Mean + std$, $Mean + 2\times{std}$, $Mean + 5\times{std}$, $Mean + 7\times{std}$, and $Mean + 9\times{std}$ as valid physical signals and used them to generate the captions. Note that the mean in this case is equal to $100$ divided by number of physical signals. As you can see in Table \ref{table:pick_sigs}, the best results are for the when pick the top $Mean + 9\times{std}$ physical signals.
%\begin{table}{r}[width=0.48\textwidth]
\begin{table}[!h]
 \caption{
Results for different approaches of picking physical signals on the $1000$ randomly selected people from validation set. We also report the average number of physical signals and average number of words in captions for each approach.}
\small
   
    \centering
    \resizebox{\linewidth}{!}{
        \begin{tabular}{@{}l cccc@{}}
        \toprule
         & mAP & ave \#sigs & ave cap len \\
         \midrule
        top1 & 25.22 & 1.0 & 22.016 &  \\
        top3 & 25.33 & 3.0 & 37.24 & \\
        top5 & 25.35 & 5.0 & 52.506 & \\
        $mean + std$ & 25.43 & 44.512 & 330.15& \\
        $mean + 3\times{std}$ & 25.53 & 12.127 & 104.702 & \\
        $mean + 5\times{std}$ & 25.32 & 5.524 & 56.184 & \\
        $mean + 7\times{std}$ & 25.47 & 3.058 & 37.816 &\\
        $mean + 9\times{std}$ & \textbf{25.54} & \textbf{1.899} & \textbf{28.986} &\\
        \bottomrule
        \end{tabular}
        
                            }
\label{table:pick_sigs}
\end{table}

% Code
% Algorithm or flowchart

\begin{table*}
\centering
\small
    \caption{The Emotion Thesaurus \cite{puglisi2019emotion} lists physical signals for numerous emotions; we included only the signals from the emotions which were synonyms of the EMOTIC labels listed here.
}
    {
        \begin{tabular}{@{}l l@{}}
        \toprule
        \textbf{EMOTIC Labels} & \textbf{The Emotion Thesaurus} \\
        \midrule
        affection & love, adoration \\
        anger & anger, resentment, rage\\
        annoyance & annoyance, irritation, impatience, frustration\\
        anticipation& anticipation\\
        aversion & disgust, hatred, reluctance  \\
        confidence & confidence, certainty, pride\\
        disapproval & contempt, scorn\\
        disconnection & indifference, boredom\\
        disquietment & nervousness, worry, anxiety\\
        doubt/confusion & confusion, doubt, skepticism\\
        embarrassment & embarrassment, guilt, shame\\
        engagement & curiosity\\
        esteem & gratitude, admiration\\
        excitement & excitement \\
        fatigue & exhaustion, lethargy\\
        fear & fear, suspicious, terror, horror\\
        happiness & happiness, amusement, joy \\
        pain & pain\\
        peace & peacefulness, satisfaction, relaxation\\
        pleasure & pleased\\
        sadness & sadness, disappointment, disappointed, discouragement\\
        sensitivity & vulnerability\\
        suffering & anguish, depression, stress, hurt\\
        surprise & surprise/shock\\
        sympathy & sympathy\\
        yearning & envy, jealousy, desire, lust\\
     
        \bottomrule
        \end{tabular}
    }
\label{table:emotic_mapping}
\end{table*}
%\end{wraptable}
\subsection{Prompts}
It is important to choose an effective prompt for LLMs. In this study, to obtain the emotion labels, first, we initially utilized the following prompt:
"\textit{<caption> From suffering, pain, aversion, disapproval, anger, fear, annoyance, fatigue, disquietment, doubt/confusion, embarrassment, disconnection, affection, confidence, engagement, happiness, peace, pleasure, esteem, excitement, anticipation, yearning, sensitivity, surprise, sadness, and sympathy, pick top labels that describe the emotion of this person.}" This prompt yielded an mAP score of 25.18 for the NarraCaps + GPT3.5 method on a randomly selected 1000 samples from the validation set. Subsequently, we modified the prompt to "\textit{From suffering, pain, aversion, disapproval, anger, fear, annoyance, fatigue, disquietment, doubt/confusion, embarrassment, disconnection, affection, confidence, engagement, happiness, peace, pleasure, esteem, excitement, anticipation, yearning, sensitivity, surprise, sadness, and sympathy, pick a set of six most likely labels that this person is feeling at the same time.}" resulting in an improved mAP of 25.50. We further refined the prompt to "\textit{From suffering(which means psychological or emotional suffering; distressed; anguished), pain(which means physical pain) , aversion(which means feeling disgust, dislike, repulsion; feeling hate), disapproval(which means feeling that something is wrong or reprehensible; contempt; hostile), anger(which mean intense displeasure or rage; furious; resentful), fear(which means feeling suspicious or afraid of danger, threat, evil or pain; horror), annoyance(which means bothered by something or someone; irritated; impatient; frustrated), fatigue(which means weariness; tiredness; sleepy), disquietment(which means nervous; worried; upset; anxious; tense; pressured; alarmed), doubt/confusion(which means difficulty to understand or decide; thinking about different options), embarrassment(which means feeling ashamed or guilty), disconnection(which means feeling not interested in the main event of the surrounding; indifferent; bored; distracted), affection(which means fond feelings; love; tenderness), confidence(which means feeling of being certain; conviction that an outcome will be favorable; encouraged; proud), engagement(which means paying attention to something; absorbed into something; curious; interested), happiness(which means feeling delighted; feeling enjoyment or amusement), peace(which means well being and relaxed; no worry; having positive thoughts or sensations; satisfied), pleasure(which means feeling of delight in the senses), esteem(which means feelings of favorable opinion or judgment; respect; admiration; gratefulness), excitement(which means feeling enthusiasm; stimulated; energetic), anticipation(which means state of looking forward; hoping on or getting prepared for possible future events), yearning(which means strong desire to have something; jealous; envious; lust), sensitivity(whcih means feeling of being physically or emotionally wounded; feeling delicate or vulnerable), surprise(which means sudden discovery of something unexpected), sadness(which means feeling unhappy, sorrow, disappointed, or discouraged), and sympathy(which means state of sharing others’ emotions, goals or troubles; supportive; compassionate), pick a set of six most likely labels that this person is feeling at the same time.}" and achieved a mAP score of 25.54. As a result, the latter prompt became the main one used in our experiments.
\subsection{Physical Signals and Environments}

Our supplementary materials include the physical signals from \cite{puglisi2019emotion} and environments from \cite{puglisi2016rural, puglisi2016urban} used to generate narrative captions, which we provide under an Attribution-Non-commercial (CC BY-NC 4.0) license following an evaluation of fair dealing. (see Table~\ref{tab:physical-signals} and \ref{tab:environments})

% All social signals 
\begin{table*}[!h]
\centering
\caption{Example Listing of Physical Signals from \cite{puglisi2019emotion}.}
\begin{tabular}{ll}
\toprule
Physical Signal Description &  \\
\midrule
Has a belly laugh & Has a clenched jaw \\
Has a bent back & Has a collapsed body posture \\
Has a bent neck & Has a confrontational stance \\
Has a bitter smile & Has a corded neck \\
Has a body that curls in on itself & Has a death grip on a purse \\
Has a bowed head & Has a head tilt \\
Has a deliberate eyebrow raise & Has a deliberate lowering of the head \\
Has a distant or empty stare & Has a downturned mouth \\
Has a downward gaze & Has a drunken behavior \\
Has a exposed the neck & Has a fight response \\
Has a flat look & Has a flush visible in the cheeks \\
Has a flushed appearance & Has a gaunt appearance \\
Has a grimace or pained look & Has a hand casually anchored on the hip \\
Has a hand flap that dismisses the person or their idea & Has a hand fluttering to the lips or neck \\
Has a hand pressing against the throat or breastbone & Has a hanging head \\
Has a hard, distinctive jaw line & Has a harried appearance \\
Has a head that tips back, exposing the neck & Has a high chin \\
Has a hunched posture & Has a mouth that curls with dislike, sneering \\
Has a pained expression & Has a pained gaze \\
Has a pained or watery gaze & Has a pained stare \\
Has a pinched expression & Has a pinched mouth \\
Has a pouty bottom lip & Has a red face and neck \\
Has a relaxed physique & Has a runny nose \\
Has a set jaw & Has a shiny face \\
Has a silly grin & Has a slack expression \\
Has a smile that appears tight & Has a stiff neck \\
Has a stony expression & Has a straight posture \\
Has a tension-filled expression & Has a thrust-out chest \\
Has a tilted-back head & Has a two-fingered salute \\
Has a welcoming stance & Has a wide grin \\
Has a wide, open stance & Has a wrinkled brow \\
Has a wrinkled nose & Has a yearning look \\
Has aggression & Has an arm hooked over the back of a chair \\
Has an expression that appears pained & Has an intense, fevered stare \\
Has an inward focus & Has an open mouth \\
Has an overall lifting of the facial countenance & Has an overall visage that glows \\
Has an unclean home, room, or office space & Has an unkempt appearance \\
Has an upturned face & Has angry tears \\
Has arms crossing in front of the chest & \\
\bottomrule
\end{tabular}
\label{tab:physical-signals}
\end{table*}

% More image and result examples

% Full breakdowns by emotion for ablations etc

% Annotation interface and description of protocol for annotators

% \begin{figure*}
%     \centering
%     \includegraphics[width = 0.99\linewidth]{latex/acci_interface.png}
%     \caption{Annotation interface for human annotators. The annotator follows the annotation procedures as follows: 1. indicate the bounding box for the subject they are annotating 2. select the perceived age, and social identity of the subject 3. Go over the lists of physical signals for eyes, mouth, face, hands, torso, and feet, and check the ones they see fit 4. Choose the correct bounding box of a subject who has interaction with the subject of interest 5. select the perceived sex, and describe the inferred relation and interaction between the two subjects 6. Describe the subject's physical surroundings. The captions generated are displayed for the annotator to review easily.}
%     \label{fig:acci_interface}
% \end{figure*}

\begin{table*}[h]
    \centering
    \resizebox{\textwidth}{!}{    
    \begin{tabular}{cccc}
        \hline
        \multicolumn{4}{c}{\textbf{Environments}} \\
        \hline
        Alley & Bank & Big City Street & Board Room \\
        Car Accident & Car Wash & Cheap Motel & Community Center \\
        Condemned Apartment Building & Construction Site & Courtroom & Elevator \\
        Emergency Room & Empty Lot & Factory & Fire Station \\
        Fitness Center & Funeral Home & Gas Station & Hair Salon \\
        Homeless Shelter & Hospital Room & Hotel Room & Juvenile Detention Center \\
        Laundromat & Library & Mechanics Shop & Military Base \\
        Morgue & Newsroom & Nursing Home & Office Cubicle \\
        Park & Parking Garage & Parking Lot & Penthouse Suite \\
        Police Station & Prison Cell & Psychiatric Ward & Public Restroom \\
        Refugee Camp & Run-Down Apartment & Sewers & Small Town Street \\
        Spa & Tattoo Parlor & Therapist Office & Underpass \\
        Vet Clinic & Waiting Room & Bakery & Bar \\
        Casual Dining Restaurant & Coffeehouse & Deli & Diner \\
        Fast Food Restaurant & Ice Cream Parlor & Pub & Antiques Shop \\
        Bazaar & Bookstore & Convenience Store & Flower Shop \\
        Grocery Store & Hardware Store & Jewelry Store & Liquor Store \\
        Pawn Shop & Pet Store & Psychics Shop & Shopping Mall \\
        Thrift Store & Used Car Dealership & Amusement Park & Art Gallery \\
        Art Studio & Ballroom & Black-Tie Event & Bowling Alley \\
        Carnival Funhouse & Casino & Circus & Golf Course \\
        Green Room & Indoor Shooting Range & Movie Theater & Museum \\
        Nightclub & Outdoor Pool & Outdoor Skating Rink & Parade \\
        Performing Arts Theater & Pool Hall & Race Track (Horses) & Rec Center \\
        Recording Studio & Rock Concert & Skate Park & Ski Resort \\
        Sporting Event Stands & Vegas Stage Show & Water Park & Zoo \\
        Airplane & Airport & Ambulance & City Bus \\
        Cruise Ship & Fishing Boat & Limousine & Marina \\
        Military Helicopter & Old Pick-Up Truck & Police Car & Submarine \\
        Subway Train & Subway Tunnel & Tank & Taxi \\
        Train Station & Truck Stop & Yacht & Attic \\
        Backyard & Basement & Bathroom & Birthday Party \\
        Block Party & Bomb Shelter & Chicken Coop & Child's Bedroom \\
        Flower Garden & Garage & Greenhouse & Group Foster Home \\
        Halloween Party & House Fire & House Party & Kitchen \\
        Living Room & Man Cave & Mansion & Motor Home \\
        Nursery & Outhouse & Patio Deck & Root Cellar \\
        Secret Passageway & Teenager Bedroom & Toolshed & Trailer Park \\
        Tree House & Underground Storm Shelter & Vegetable Patch & Wake \\
        Wine Cellar & Workshop & Boarding School & Custodial Supply Room \\
        Dorm Room & Elementary School Classroom & Gymnasium & High School Cafeteria \\
        High School Hallway & Locker Room & Playground & Preschool \\
        Principal Office & Prom & School Bus & Science Lab \\
        Teacher Lounge & University Lecture Hall & University Quad & Abandoned Mine \\
        Ancient Ruins & Archery Range & Barn & Beach Party \\
        Campsite & Church & Country Road & County Fair \\
        Farmer Market & Graveyard & Hunting Cabin & Landfill \\
        Lighthouse & Mausoleum & Orchard & Pasture \\
        Quarry & Ranch & Rodeo & Salvage Yard \\
        Slaughterhouse & Summer Camp & Taxidermist & Wedding Reception \\
        Winery & Arctic Tundra & Badlands & Beach \\
        Canyon & Cave & Creek & Desert \\
        Forest & Grotto & Hiking Trail & Hot Springs \\
        Lake & Marsh & Meadow & Moors \\
        Mountains & Ocean & Pond & Rainforest \\
        River & Swamp & Tropical Island & Waterfall \\
        \hline
    \end{tabular}
    }
    \caption{Example listing of environments from \cite{puglisi2016rural, puglisi2016urban}.}
    \label{tab:environments}
\end{table*}
